# Supplementary material for: Inform the uninformed: Improving Online Informed Consent Reading with an AI-Powered Chatbot
Source: arXiv:2302.00832 source file (2023-02-02)
Supplement: Supplementary file 1 [file 06_appendix.tex]

\appendix
\onecolumn
\section{Appendix}
\subsection{Manipulation Checks}
To validate our problematic social media use survey design with different risk levels, we asked participants to rate their perceived sensitivity and risk regarding the survey upon completion. Both ratings are on 5-point Likert scales. The results confirm our design. Participants in the Low-risk condition felt the survey was the least sensitive, whereas the participants in the High-risk condition perceived the survey as the most sensitive (Low: M = 1.64, SD = 0.83; Medium: M = 1.92, SD = 1.27; High: M = 3.13, SD = 1.31). The ANOVA analysis with the Tukey method suggests that, for the perceived data sensitivity, the differences between the three risk levels are statistically significant (High-Low: p < 0.01; Medium-Low: p < 0.01; High-Medium: p < 0.01).

Participants in the Low-risk condition report the lowest level of perceived risk for the survey, whereas participants in the High-risk condition report the highest (Low: M = 1.66. SD = 0.67; Medium: M = 2.23, SD = 1.11; High: M = 2.71, SD = 1.11). Through ANOVA analysis with Tukey method, we found the differences between Low and High and between High and Medium are statistically significant, but the difference between Low and Medium is not (High-Low: p < 0.01; Medium-Low: p = 0.25; High-Medium: p < 0.01). Both manipulation checks suggested our manipulation of the survey's perceived level of risk was successful.

\subsection{Bayesian Model Specifications}
\label{sec:bms}
In this section, we provide details of the set up of our Bayesian models. In a Bayesian formulation, we define a likelihood function to model the dependent variable that represents the modeler's view of the data, not a claim about the world \cite{mcelreath2020statistical}.  The likelihood function is parametric, meaning that we treat each model parameter as a random variable drawn from another distribution with parameters (its prior distribution).  We use weakly informative priors to make conservative estimations and encode skepticism but not impossibility towards large effect sizes.  For all the Bayesian models discussed in this section, all parameters achieved a Gelman-Rubin statistic (a measure of MCMC convergence) of 1.0, indicating that the multiple sampling chains converged. Traceplots that visualize sampling results are available in the supplementary materials.

All of our Bayesian models (except the SEM model) share the same predictor (consent method) and covariates (risk level and demographics). We use partially pooled varying intercepts to describe the effect of consent method and gender, making the models hierarchical. We describe the parameters for the variables below, with $i$ representing the i-th participant. 

    \begin{description}
        \item $\bm{C_i}$: Varying intercept for the effect of the consent method used by participant $i$.
        \item $\bm{\beta_R\sum_{n=0}^{R_{[i]}-1}\delta_R}$: Slope for risk level of participant $i$ as an ordinal variable.
        \item $\bm{G_i}$: Varying intercept for the effect of gender of participant $i$.
        \item $\bm{\beta_A\sum_{n=0}^{A_{[i]}-1}\delta_A}$: Slope for the age level of participant $i$ as an ordinal variable.
        \item $\bm{\beta_E\sum_{n=0}^{E_{[i]}-1}\delta_E}$: Slope for the education level of participant $i$ as an ordinal variable.
        \item $\bm{\beta_I\sum_{n=0}^{I_{[i]}-1}\delta_I}$: Slope for the income level of participant $i$ as an ordinal variable.
    \end{description}

We define the linear model made up of the predictor and covariates as follows:

    \begin{align*}
        LM_{i} &= C_{[i]} + \beta_R\sum_{n=0}^{R[i]-1}\delta_R + G_{[i]} + \beta_A\sum_{n=0}^{A[i]-1}\delta_A + \beta_E\sum_{n=0}^{E[i]-1}\delta_E + \beta_I\sum_{n=0}^{I[i]-1}\delta_I
    \end{align*}

The priors we selected for the parameters are as follows. We will specify the hyper priors within each model in the upcoming sections.

    \begin{align*}
        C_i &\sim N(\bar{\mu}, \bar{\sigma}) &\text{Prior for each consent method}\\
        \beta_R &\sim N(\mu_{\beta}, \sigma_{\beta}) &\text{Prior for slope of risk level}\\
        \delta_R &\sim Dirichlet(2) &\text{Prior for the cutpoints of ordinal risk levels}\\
        G_i &\sim N(\bar{\mu}, \bar{\sigma}) &\text{Prior for each gender}\\
        \beta_A &\sim N(\mu_{\beta}, \sigma_{\beta}) &\text{Prior for slope of age level}\\
        \delta_A &\sim Dirichlet(2) &\text{Prior for the cutpoints of ordinal age levels}\\
        \beta_E &\sim N(\mu_{\beta}, \sigma_{\beta}) &\text{Prior for slope of education level}\\
        \delta_E &\sim Dirichlet(2) &\text{Prior for the cutpoints of ordinal education levels}\\
        \beta_I &\sim N(\mu_{\beta}, \sigma_{\beta}) &\text{Prior for slope of income level}\\
        \delta_I &\sim Dirichlet(2) &\text{Prior for the cutpoints of ordinal income levels}\\
    \end{align*}

As described in Section \ref{data_analysis}, we built two kinds of Bayesian models, a linear regression model and an ordered logistic regression model. Next, we detail the formulation of these two models.

\subsubsection{Linear regression model}
\label{sec:bml}
    We model the dependent variable as a Normal distribution.

    \begin{align*}
        DV_i &\sim N(\mu_i, \sigma_i)\\
        \mu_i &= \alpha_{\mu} + LM_{i}\\
        \sigma_i &= \alpha_{\sigma} + C_{\sigma_i}\\
    \end{align*}

    The additional priors for parameters new in the equations above are as follows:

    \begin{align*}
        \alpha_{\mu} &\sim N(\mu_{DV}, \sigma_{DV}*0.1) &\text{Prior for the intercept of } \mu \\
        \alpha_{\sigma} &\sim N(\sigma_{DV}, \sigma_{DV}*0.1) &\text{Prior for the intercept of } \sigma \\
        C_{\sigma_i} &\sim N(\bar{\mu}, \bar{\sigma}) &\text{Prior for the effect of each consent method on } \sigma
    \end{align*}

    For hyper priors, we set $\bar{\mu} \sim N(0, 1)$ and $\bar{\sigma} \sim Exp(1)$. For the priors of slopes $\beta$, we set $\mu_{\beta} = 0$ and $\sigma_{\beta} = 1$. For the priors of intercepts $\alpha$, $\mu_{DV}$ and $\sigma_{DV}$ represents the mean and standard deviation of the dependent variable observed in our data.

\subsubsection{Ordered logistic model}
\label{sec:bmo}
    In an ordered logistic model, we model the logit of the cumulative probability function of the dependent variable as a linear regression. Let $q_k$ be the cumulative probability of getting a value of $k$ or lower on the ordinal scale.

    \begin{align*}
        logit(q_k) &= \alpha_k - \phi_i\\
        \phi_i &= LM_{i}\\
        \alpha_k &\sim N(0, 1)
    \end{align*}

    For hyper priors, we set $\bar{\mu} \sim N(0, 0.25)$ and $\bar{\sigma} \sim Exp(1)$. For the priors of slopes $\beta$, we set $\mu_{\beta} = 0$ and $\sigma_{\beta} = 0.25$.
